# Supplementary material for: Robust Quantity-Aware Aggregation for Federated Learning
Source: arXiv:2205.10848 source file (2023-07-26)
Supplement: Supplementary file 1 [file L1-Krum.tex]

\section{Base Aggregation}
\subsection{Proof of Proposition 1}
\label{sec:proof-pro1}

\textit{Proof.} Without loss of generality, we assume malicious vectors are placed in the last $m$ positions in the arguments of the $\normlone$-based Krum, i.e., $\textbf{g} = \normlone\text{-Krum}(\textbf{g}^1, ..., \textbf{g}^{n-m}, ..., \textbf{g}^{n})$. For each index $i$, we denote the number of benign indexes j such that $i \to j$ as $\delta_c(i)$, and the number of malicious indexes j such that $i \to j$ as $\delta_b(i)$.
We have
\begin{equation}
    \begin{aligned}
        \delta_c(i) + \delta_b(i) &= n - m - 2, \\
        n-2m-2 \leq \delta_c(i) &\leq n - m - 2, \\
        \delta_b(i) &\leq m. \\
    \end{aligned}
\end{equation}

We denote the $i_*$ as the index selected by $L_1$-Krum.
\begin{equation}
    \begin{aligned}
    \E[||\textbf{g} - \boldsymbol \mu ||_1] &\leq \sum_{\text{benign $i$}} \E[||\textbf{g}^i -\boldsymbol \mu||_1 \mathbb{I}(i_* = i)] \\
    &+ \sum_{\text{malicious $k$}} \E[||\textbf{g}^k -\boldsymbol \mu||_1 \mathbb{I}(i_* = k)],
    \end{aligned}
    \label{eq:pro1-benign-mal}
\end{equation}
where $\mathbb{I}$ denotes the indicator function.
We focus on the case that $i_* = i$ for some correct index $i$ in Equation~\ref{eq:pro1-benign-mal}.
We first prove the following lemma.
\begin{lemma}
Let $\textbf{g}^1$, ..., $\textbf{g}^{n}$ be independent identically distributed random vectors with the same quantity $q$, where $\textbf{g}^i \subseteq \mathbb{R}^d$, and $\E\, [\textbf{g}^i] =\boldsymbol \mu$.
Supposing that Assumption~\ref{assume:sample-sub-exp} holds,
then we have
\begin{equation}
\E[\max_{i}||\textbf{g}^i -\boldsymbol \mu||_1]\leq \sqrt{2 \ln 2n} ||\boldsymbol \sigma||_1 / \sqrt{q},
\end{equation}
\label{lemma:exp-sub-exp-mu}
\end{lemma}
where $\boldsymbol \sigma$ is a d-dimensional vector denoted as $[\sigma_1, ..., \sigma_{d}]$.

\textit{Proof.} See Appendix~\ref{sec:proof-lemma-exp-sub-exp-mu}.

Applying Lemma~\ref{lemma:exp-sub-exp-mu} on the first term of Equation~\ref{eq:pro1-benign-mal}, we obtain
\begin{equation}
    \begin{aligned}
    \sum_{\text{benign $i$}} \E[||\textbf{g}^i -\boldsymbol \mu||_1 \mathbb{I}(i_* = i)] &\leq \E[\max_{\text{benign $i$ }}||\textbf{g}^i -\boldsymbol \mu||_1] \\
    & \leq  \sqrt{2 \ln 2(n-m)} ||\boldsymbol \sigma||_1 / \sqrt{q}.
    \end{aligned}
\end{equation}

Next we focus on the case that $i_* = k$ for some malicious index $k$ in Equation~\ref{eq:pro1-benign-mal}.
\begin{equation}
    \begin{aligned}
        &\sum_{\text{malicious } k} \E[||\textbf{g}^k -\boldsymbol \mu||_1  \mathbb{I}(i_* = k)] \\
        &\leq \sum_{\text{malicious }k}\E[||\boldsymbol \mu - \frac{1}{\delta_c(k)}\sum_{j:k \to j \atop \text{benign $j$}}\textbf{g}^j||_1\mathbb{I}(i_* = k)] \\
        &+ \sum_{\text{malicious }k}\E[||\textbf{g}^k -\frac{1}{\delta_c(k)}\sum_{j:k \to j \atop \text{benign $j$}}\textbf{g}^j ||_1\mathbb{I}(i_* = k)] \\
        &\leq \E[\max_{\text{malicious }k}\frac{1}{\delta_c(k)}\sum_{\text{benign $j$}}||\boldsymbol \mu - \textbf{g}^j||_1] \\
        &+ \sum_{\text{malicious }k}\E[||\textbf{g}^k -\frac{1}{\delta_c(k)}\sum_{j:k \to j \atop \text{benign $j$}}\textbf{g}^j ||_1\mathbb{I}(i_* = k)] \\
    \end{aligned}
    \label{eq:prob1-mal}
\end{equation}

If $k$ is selected by the $\normlone$-based Krum, it implies for any correct index $i$
\begin{equation}
\begin{aligned}
    &\sum_{\text{malicious }k}\mathbb{I}(i_* = k)[\sum_{j:k \to j \atop \text{benign $j$}}||\textbf{g}^k - \textbf{g}^j||_1 + \sum_{j:k \to j \atop \text{malicious $j$}}||\textbf{g}^k - \textbf{g}^j||_1] \\
    &\leq \sum_{j:i \to j \atop \text{benign $j$}}||\textbf{g}^i - \textbf{g}^j||_1 + \sum_{j:i \to j \atop \text{malicious $j$}}||\textbf{g}^i - \textbf{g}^j||_1.
\end{aligned}
\end{equation}

Therefore, for any correct index $i$
\begin{equation}
    \begin{aligned}
        &\sum_{\text{malicious }k}||\textbf{g}^k -\frac{1}{\delta_c(k)}\sum_{j:k \to j \atop \text{benign $j$}}\textbf{g}^j ||_1\mathbb{I}(i_* = k) \\
        &\leq \sum_{\text{malicious }k}\frac{\mathbb{I}(i_* = k)}{\delta_c(k)} \sum_{j:k \to j \atop \text{benign $j$}}||\textbf{g}^k - \textbf{g}^j||_1 \\
        &\leq \frac{1}{n-2m-2}\sum_{j:i \to j \atop \text{benign $j$}}||\textbf{g}^i - \textbf{g}^j||_1 + \frac{1}{n-2m-2}\sum_{j:i \to j \atop \text{malicious $j$}}||\textbf{g}^i - \textbf{g}^j||_1.
    \end{aligned}
    \label{eq:pro1-mal}
\end{equation}

We focus on the second term of Equation~\ref{eq:pro1-mal}. Since any correct index $i$ has $n-m-2$ neighbors and $m+1$ non-neighbors.
There exists at least one benign index $\varsigma(i)$, which is farther from $i$ than any of its neighbors.
Therefore, $\forall j:\ i \to \text{malicious } j $, $||\textbf{g}^i - \textbf{g}^j||_1 \leq ||\textbf{g}^i - \textbf{g}^{\varsigma(i)}||_1$.
Then we have
\begin{equation}
    \begin{aligned}
        &\sum_{\text{malicious }k}||\textbf{g}^k -\frac{1}{\delta_c(k)}\sum_{j:k \to j \atop \text{benign $j$}}\textbf{g}^j||_1 \mathbb{I}(i_* = k)\\
        &\leq \frac{1}{n-2m-2}\sum_{j:i \to j \atop \text{benign $j$}}||\textbf{g}^i - \textbf{g}^j||_1 + \frac{\delta_b(i)}{n-2m-2}||\textbf{g}^i - \textbf{g}^{\varsigma(i)}||_1.
    \end{aligned}
\end{equation}

\begin{equation}
    \begin{aligned}
        &\sum_{\text{malicious }k}\E[||\textbf{g}^k -\frac{1}{\delta_c(k)}\sum_{j:k \to j \atop \text{benign $j$}}\textbf{g}^j||_1 \mathbb{I}(i_* = k)]\\
        &\leq \frac{2\sqrt{2\ln 2}(n-m)}{(n-2m-2)\sqrt{q}}||\boldsymbol \sigma||_1 + \frac{\delta_b(i)}{n-2m-2}\sum_{\text{benign $j$}\neq i}\E[||\textbf{g}^i - \textbf{g}^{j}||_1\mathbb{I}(\varsigma(i) = j)] \\
        &\leq \frac{2\sqrt{2\ln 2}(n-m)}{(n-2m-2)\sqrt{q}}||\boldsymbol \sigma||_1 + \frac{\delta_b(i)}{n-2m-2}\E\max_{\text{benign $j$}\neq i}||\textbf{g}^i - \textbf{g}^{j}||_1 \\
        % &\leq \frac{\delta_c(i)}{\delta_c(k)}\sqrt{\frac{2}{\pi}}||\boldsymbol \sigma||_1 + 2\frac{\delta_b(k)}{\delta_c(k)}\sqrt{2 \ln 2(n-f)} ||\boldsymbol \sigma||_1 \\
        &\leq \frac{2\sqrt{2\ln 2}(n-m) + 2m\sqrt{2 \ln 2(n-m)}}{(n-2m-2)\sqrt{q}}  ||\boldsymbol \sigma||_1.
    \end{aligned}
    \label{eq:mal-minus-benign}
\end{equation}

Putting Equation~\ref{eq:mal-minus-benign} back to Equation~\ref{eq:prob1-mal}, we obtain
\begin{equation}
    \begin{aligned}
        \sum_{\text{malicious } k} \E[||\textbf{g}^k -\boldsymbol \mu||_1 \mathbb{I}(i_* = k)] 
        &\leq \frac{3\sqrt{2\ln 2}(n-m) + 2m\sqrt{2 \ln 2(n-m)}}{(n-2m-2)\sqrt{q}}  ||\boldsymbol \sigma||_1
    \end{aligned}
\end{equation}
Putting everything back together, we get
\begin{equation}
\E [||\textbf{g} - \boldsymbol \mu ||_1] \leq  \frac{3\sqrt{2\ln 2}(n-m) + (n-2)\sqrt{2 \ln 2(n-m)}}{(n-2m-2)\sqrt{q}} ||\boldsymbol \sigma||_1.
\end{equation}

\subsection{Proof of Lemma 2}
\label{sec:proof-lemma-exp-sub-exp-mu}

\textit{Proof.}
We first convert the problem of computing the expectation of the maximum of the $\normlone$ norm of the d-dimensional vectors into the problem of computing expectations of the maximum of each dimension of the d-dimensional vectors.
\begin{equation}
\begin{aligned}
\label{eq:lemma2-max}
\E[\max_{i}||\textbf{g}^i -\boldsymbol \mu||_1] &= \E[\max_{i}\sum_{k\in\{1,...,d\}}|g_k^i - \mu_k|] \\
&\leq \sum_{k\in\{1,...,d\}}\E[\max_{i}|g_k^i - \mu_k|].
\end{aligned} 
\end{equation}

Following the same logic in Appendix~\ref{sec:proof-lemma1}, it is easy to prove $g_k^i$ is sub-exponential with parameters $(\frac{v_k^2}{q}, \frac{\alpha_k}{q})$, where $v_k = \sigma_k$ and $\alpha_k \leq \frac{\sigma_k}{\sqrt{2\ln 2n}}$.
% From Assumption~\ref{assume:sub-exp}, we know $g_k^i \sim \mathcal{N}(\mu_k, \sigma_k^2)$.
% We then denote $x_k^i = g_k^i - \mu_k$, where $x_k^i \sim \mathcal{N}(0, \sigma_k^2)$.
% Then we have
% \begin{equation}
% z_k = \max_{i}|g_k^i - \mu_k| = \max_{i}|x_k^i|.
% \end{equation}
Define $x_k^i = g_k^i - \mu_k$.
Denote a list of values $X=\{x_k^1, -x_k^1, ..., x_k^n, -x_k^n\}$, and $z_k = \max_{i}|g_k^i - \mu_k| = \max_{x \in X}x$.
We then obtain
\begin{equation}
\begin{aligned}
e^{\lambda\E[z_k]} &\leq \E [e^{\lambda z_k}] = \E [\max_{x\in X}e^{\lambda x}] \leq \sum_{x \in X} \E [e^{\lambda x}] \leq 2n e^{\frac{\lambda^2 \sigma_k^2}{2q}}.
\end{aligned} 
\end{equation}
\begin{equation}
\E[z_k] \leq \frac{\ln 2n}{\lambda} + \frac{\lambda \sigma_k^2}{2q}.
\end{equation}

Setting $\lambda = \frac{\sqrt{2q \ln 2n}}{\sigma_k} < \frac{q}{\alpha_k}$, we can get
\begin{equation}
~\label{eq:lemma2-lnn}
\E[z_k] \leq \sigma_k \sqrt{2 \ln 2n} / \sqrt{q}.
\end{equation}

Putting Equation~\ref{eq:lemma2-lnn} back to Equation~\ref{eq:lemma2-max}, we obtain 
\begin{equation}
\E [\max_{i}||\textbf{g}^i -\boldsymbol \mu||_1]\leq \sqrt{2 \ln 2n} ||\boldsymbol \sigma||_1 / \sqrt{q},
\end{equation}
where $\boldsymbol \sigma$ is a d-dimensional vector denoted as $[\sigma_1, ..., \sigma_{d}]$.

\subsection{Proof of Theorem 1}
\label{sec:proof-of-non-convex}
\textit{Proof.}
% Using the smoothness of $F(\cdot)$ and setting $\eta=1/L_F$, Equation~\ref{eq:smoothness} holds.
Following the proof of Theorem 2 in~\cite{yin2018byzantine}, using the smoothness of $F(\cdot)$ and setting $\eta=1/L_F$, we have
\begin{equation}
    F(\textbf{w}_{t+1}) \leq F(\textbf{w}_t) - \frac{1}{2L_F}||\nabla F(\textbf{w}_t)||_2^2 + \frac{1}{2L_F}||\textbf{g}_t - \nabla F(\textbf{w}_t)||_2^2.
\label{eq:smoothness}
\end{equation}

% According to Proposition~\ref{prop:l1-br}, we obtain
% \begin{equation}
%     \E F(\textbf{w}^{t+1}) \leq \E F(\textbf{w}^t) - \frac{1}{2L_F}\E||\nabla F(\textbf{w}^t)||_2^2 + \frac{1}{2L_F}(\zeta(n, m)||\boldsymbol \sigma||_1)^2.
% \label{eq:smoothness}
% \end{equation}

According to Proposition~\ref{prop:l1-br}, we further obtain
\begin{equation}
    \E [F(\textbf{w}_{t+1}) - F(\textbf{w}^*)] \leq \E [F(\textbf{w}_{t}) - F(\textbf{w}^*)] - \frac{1}{2L_F}\E[||\nabla F(\textbf{w}_t)||_2^2] + \frac{1}{2L_F}(\zeta(n, m)||\boldsymbol \sigma||_1)^2. 
    \label{eq:smoothness-con-convex}
\end{equation}
Sum up Equation~\ref{eq:smoothness-con-convex}, we have 
\begin{equation}
    \begin{aligned}
         0 &\leq \E [F(\textbf{w}_{T}) - F(\textbf{w}^*)] \\ &\leq \E [F(\textbf{w}^{0}) - F(\textbf{w}^*)] - \frac{1}{2L_F}\sum_{t=0}^{T-1}\E[||\nabla F(\textbf{w}_t)||_2^2] + \frac{T}{2L_F}(\zeta(n, m)||\boldsymbol \sigma||_1)^2,
    \end{aligned}
\end{equation}
which implies
\begin{equation}
    \min_{t=0,...,T}\E[||\nabla F(\textbf{w}_t)||_2^2] \leq \frac{2L_F}{T}\E [F(\textbf{w}_{0}) - F(\textbf{w}^*)] + (\zeta(n, m)||\boldsymbol \sigma||_1)^2.
\end{equation}

\subsection{Proof of Lemma 1}
\label{sec:proof-lemma1}
\textit{Proof.}
As defined in Section~\ref{sec:prob-define}, we have $g_k^i = \frac{1}{q^i} \sum_{z \in \mathcal{D}_i} \partial_k f(\textbf{w};z)$.
Therefore, we can obtain
\begin{equation}
    \begin{aligned}
    \E[g_k^i] = \frac{1}{q^i} \sum_{z \in \mathcal{D}_i} \E[\partial_kf(\textbf{w};z)] = \mu_k,
    \end{aligned}
\end{equation}
\begin{equation}
    \begin{aligned}
    \E[(g_k^i - \mu_k))^2] &= \E[(\frac{1}{q^i} \sum_{z \in \mathcal{D}_i} \partial_kf(\textbf{w};z) - \mu_k)^2] \\
    &= \frac{1}{(q^i)^2} \sum_{z \in \mathcal{D}_i} \E[(\partial_kf(\textbf{w};z) - \mu_k)^2] = \frac{\sigma_k^2}{q^i}.
    \end{aligned}
\end{equation}

Since $\partial_k f(\textbf{w};z)$ is sub-exponential with parameters $(v_k^2, \alpha_k)$, we have
\begin{equation}
    \begin{aligned}
    e^{\frac{\lambda}{q^i}\sum_{z \in \mathcal{D}_i} (\partial_k f(\textbf{w};z) - \mu_k)} \leq e^{\frac{1}{2q^i}v^2\lambda^2},
    \end{aligned}
\end{equation}
when $\lambda \leq \frac{q^i}{\alpha_k}$.
It shows $g_k^i$ is sub-exponential with parameters $(\frac{v_k^2}{q^i}, \frac{\alpha_k}{q^i})$, where $v_k = \sigma_k$ and $\alpha_k \leq \frac{\sigma_k}{\sqrt{2\ln 2n}}$. $n$ is the number of clients sampled by server in each round.

Follow the same logic in Lemma~\ref{lemma:exp-sub-exp-mu}, we have
\begin{equation}
    \begin{aligned}
    \E[|g_k^i - \mu_k|] &\leq \sqrt{2\ln 2} \frac{\sigma_k}{\sqrt{q^i}}.
    \end{aligned}
\end{equation}

Obviously, we can obtain
\begin{equation}
    \begin{aligned}
        \E[\textbf{g}^i] = \boldsymbol \mu, \;
        \E[\sqrt{q^i}||\textbf{g}^i - \boldsymbol \mu||_1] \leq \sqrt{2\ln 2}||\boldsymbol \sigma||_1.
    \end{aligned}
\end{equation}

\subsection{Proof of Example 1}
\label{sec:proof-l1-qkrum}
% change to use an example to show the error of  L1-Qkrum
\textit{Proof.}
Since benign updates are independently distributed and are with the same quantities $q$, the probability of each benign updates being selected is the same.
Therefore, due to $\boldsymbol \mu=0$ we can have
\begin{equation}
    \begin{aligned}
        \E[\sqrt{q}||\textbf{g} - \boldsymbol \mu||_1] &= \E[\sqrt{q_m}||\textbf{g}_m - \boldsymbol \mu||_1]p_m + \E[\sqrt{q_b}||\textbf{g}^1 - \boldsymbol \mu||_1](1-p_m) 
        \geq \sqrt{q_m}|\epsilon| p_m.
    \end{aligned}
\end{equation}

In $\normlone$-based QKrum, since whether $\textbf{g}_m$ is selected is only related to the distance between $\textbf{g}_m$ and its neighbors, $p_m$ is irrelevant with $q_m$.
Therefore, we can treat $p_m$ as a constant. 
When $q_m = (k/(p_m\cdot \epsilon))^2$, we have
\begin{equation}
    \begin{aligned}
        \E[\sqrt{q}||\textbf{g} - \boldsymbol \mu||_1] \geq k,
    \end{aligned}
\end{equation}
where $k$ can be arbitrary positive value.
